# Supplementary material for: Last-Layer Fairness Fine-tuning is Simple and Effective for Neural Networks
Source: arXiv:2304.03935 source file (2023-07-14)
Supplement: Supplementary file 1 [file appendix.tex]

\begin{table}[ht]
\centering
\setlength{\tabcolsep}{4pt}
\begin{tabular}{|c|c|c|c|}
\hline
  {(train/val/test)} & Blonde Hair & Non-blonde Hair   & Total \\ \hline

  Male & 1,387/182/180 & 66,874/8,276/7,535 & 68,261/8,458/7,715   \\ \hline
  Female & 22,880/2,874/2,480 & 71,629/8,535/9,767 & 94,509/11,409/12,247 \\   \hline
  Total  & 24,267/3,056/2,660 & 138,503/16,811/17,302 & 162,770/19,867/19,962 \\  \hline
\end{tabular}
\caption{\textbf{CelebA (Hair Color) statistics.} }
\label{tab:datasets1}
\end{table}
% \begin{table}[ht]
% \centering
% \setlength{\tabcolsep}{4pt}
% \begin{tabular}{|c|c|c|c|}
% \hline
%   {(train/val/test)} & Pale Skin & Non-pale Skin   & Total \\ \hline

%   Male & 1,695/195/166 & 66,566/8,263/7,549 & 68,261/8,458/7,715   \\ \hline
%   Non-male & 5,310/661/674 & 89,199/10,748/11,573 & 94,509/11,409/12,247 \\   \hline
%   Total  & 7,005/856/840 & 155,765/19,011/19,122 & 162,770/19,867/19,962 \\  \hline
% \end{tabular}
% \caption{\textbf{CelebA (Skin Color) statistics.} }
% \label{tab:datasets2}
% \end{table}
\begin{table}[ht]
\centering
\setlength{\tabcolsep}{4pt}
\begin{tabular}{|c|c|c|c|}
\hline
  {(train/val/test)} & Consolidation & Non-consolidation   & Total \\ \hline

  Male & 75,867/13,276/5,793 & 49,705/8,698/3,755 & 125,572/21,974/9,548   \\ \hline
  Female & 51,469/9,007/3,926 & 33,965/5,944/2,589 & 86,434/14,951/6,515 \\   \hline
  Total  & 127,336/22,283/9,719 & 83,670/14,642/6,344 & 211,006/36,925/16,063 \\  \hline
\end{tabular}
\caption{\textbf{CheXpert statistics.} }
\label{tab:datasets2}
\end{table}
